# Supplementary material for: Comprehensible Artificial Intelligence on Knowledge Graphs: A survey
Source: arXiv:2404.03499 source file (2024-04-04)
Supplement: Supplementary file 1 [file appendix.tex]

%-------------------------------------------
\section*{Appendix}\label{sec:ap}
%-------------------------------------------
\subsection*{Appendix 1}\label{subsec:ap_1}

\begin{figure}[p]

\centering
\includegraphics[width=1.3\textwidth, angle =90 ]{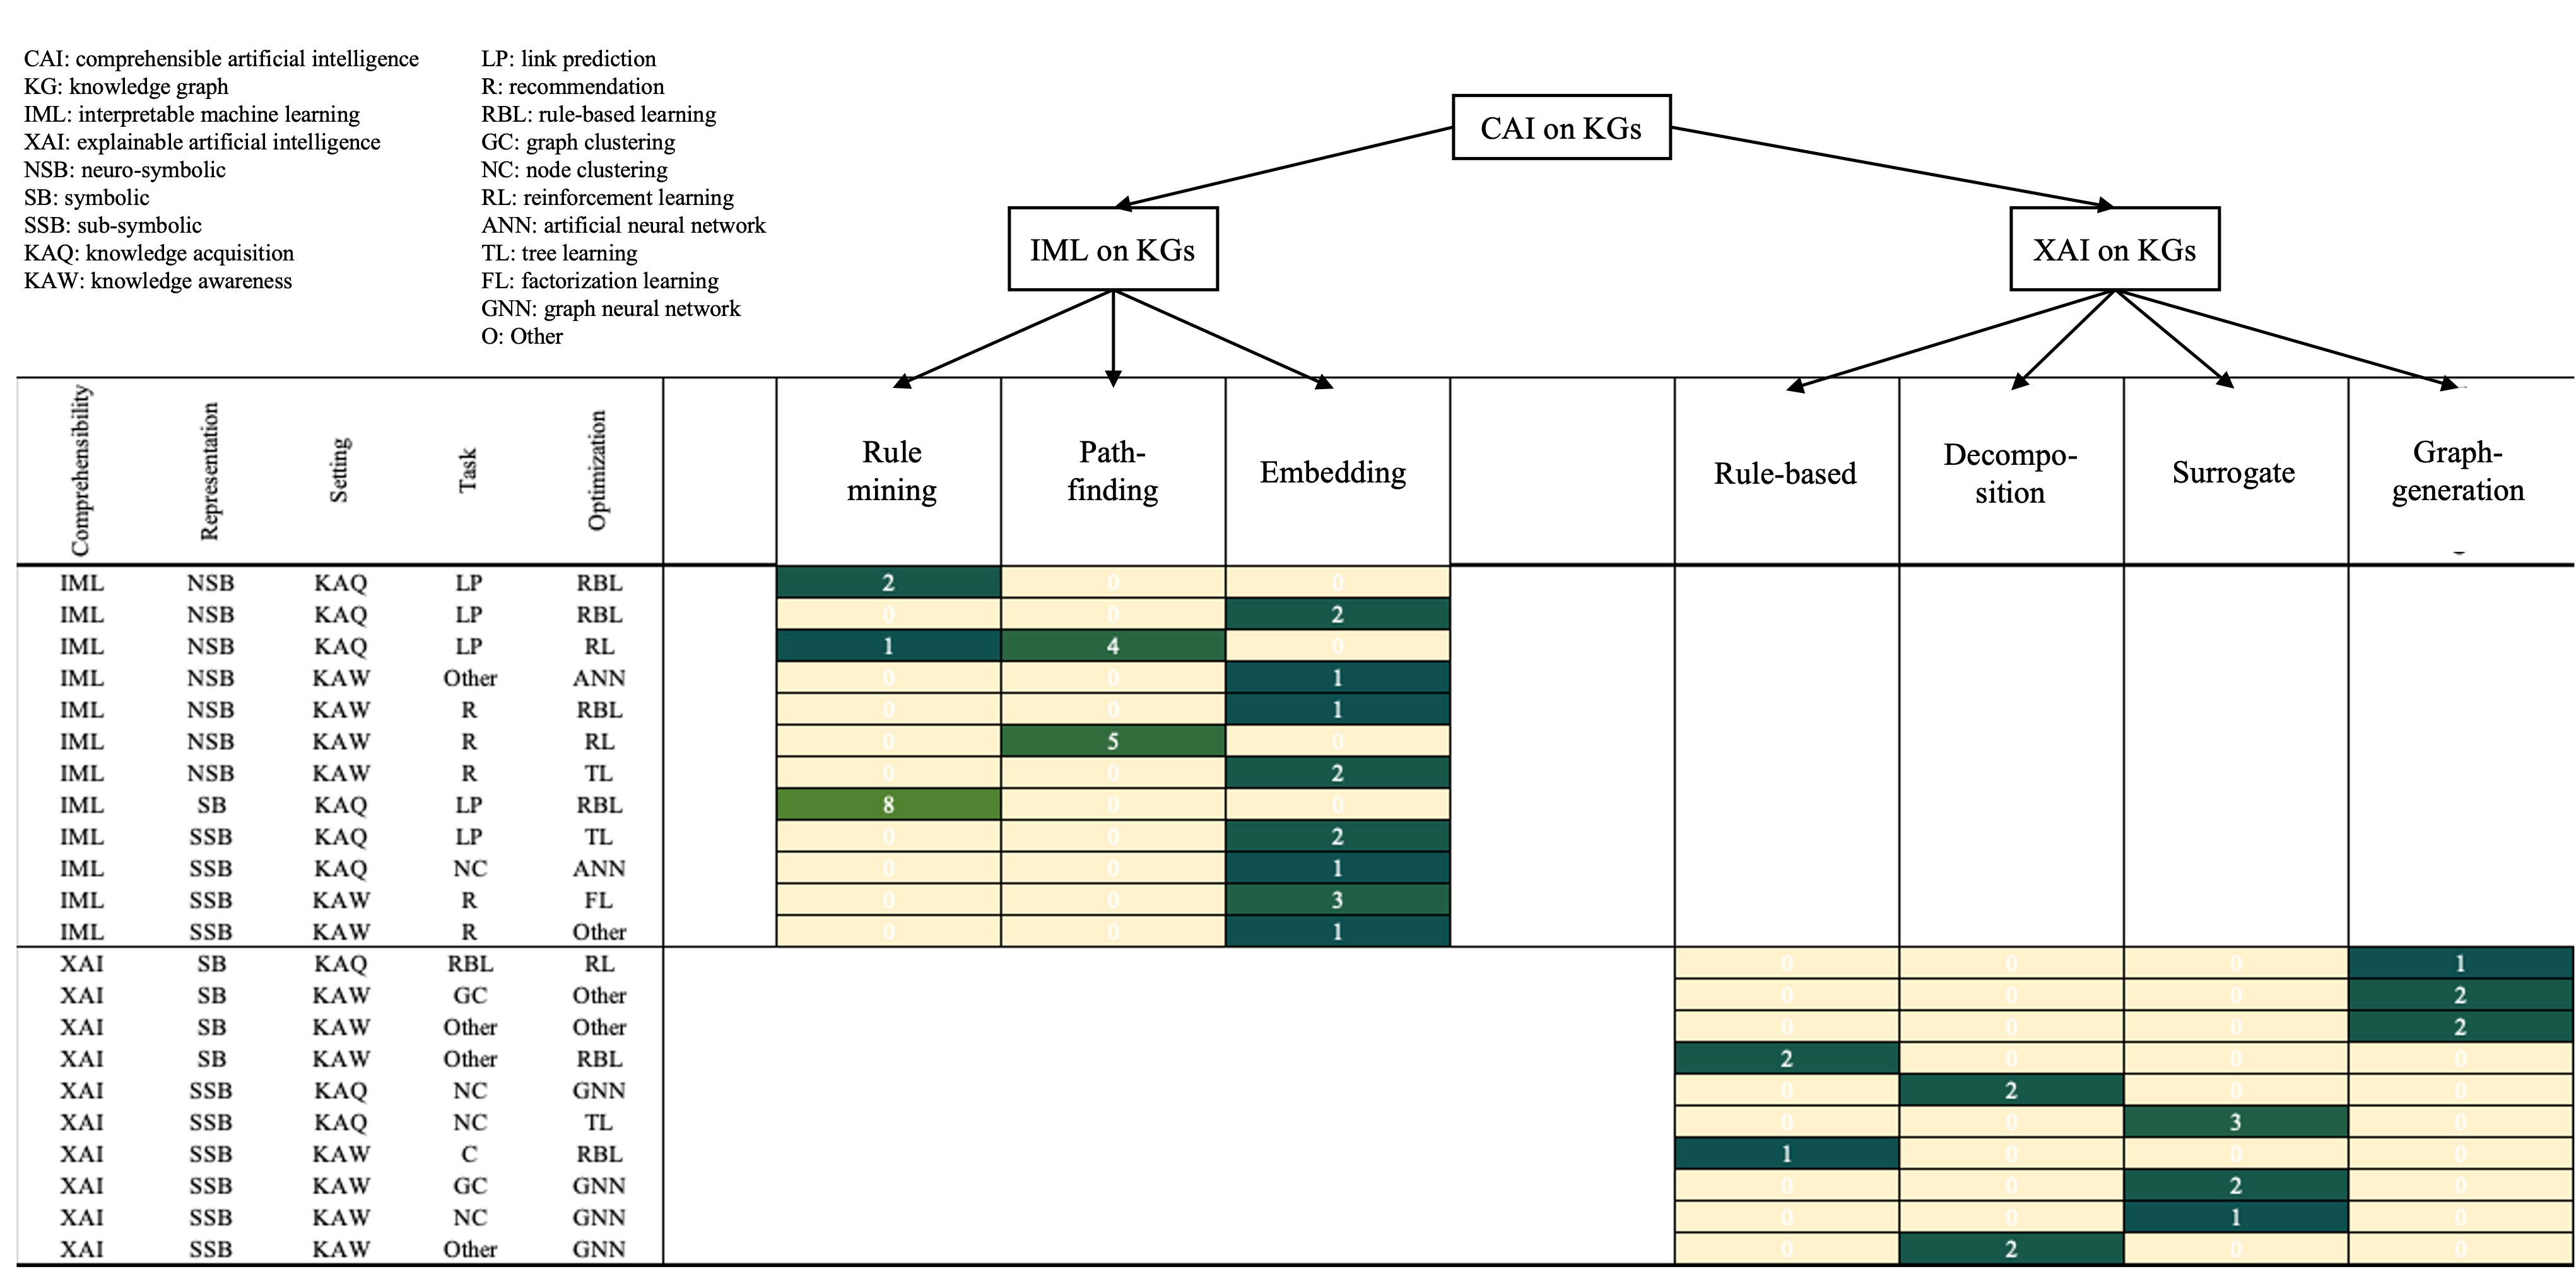}
\caption{Box plot of number of positions sent per iteration using this scheme}
\label{fig:awesome_image}

\end{figure}
